# Supplementary material for: Addressing Data Heterogeneity in Decentralized Learning via Topological Pre-processing
Source: arXiv:2212.08743 source file (2022-12-16)
Supplement: Supplementary file 1 [file 08_supplementary_materials.tex]

\newpage
\onecolumn
\section{\centering{Supplementary experimental results}}

\label{sec:sup}

\subsection{Summary}
In supplementary materials, we also exhibit the situation where \proj is not outperform baselines. This is reasonable, since every method have their own strength and weakness, there is no superior solution can universal in all possible FL settings.
Again, we summarized scenarios that \proj shows in advanced: 
1. bandwidth matters.
2. public data available  
3. edge devices are resource limited.
4. large scale.

\subsection{Learning Efficiency}

\subsection{Communication Cost}

\subsection{Ablation Study}

\subsection{Difference}
